# Supplementary material for: Input-Output Theory with Quantum Pulses
Source: arXiv:1902.09833 ancillary file (2019-06-24)
Supplement: Supplementary file 1 [file InputOutputWithQuantumPulses_Supp_Mat.pdf]

# Input-Output Theory with Quantum Pulses: Supplemental Materials

Alexander Holm Kiilerich* and Klaus Mølmer†
*Department of Physics and Astronomy, Aarhus University, Ny Munkegade 120, DK 8000 Aarhus C. Denmark*

(Dated: May 28, 2019)

## I. MULTIPLE OUTPUT AND INPUT MODES

The output field may occupy several ($m$) orthogonal modes $\{v_i(t)\}_{i=1}^m$ and to extend our formalism to multiple output modes, we assume that after the first virtual cavity, which perfectly absorbs the mode $v_1(t)$, the field is serially reflected on a sequence of virtual cavities. They each have their own coupling strength $g_{v_i}(t)$, designed such that the quantum state content of the mode $v_i(t)$ is precisely captured by the internal field $\hat{a}_{v_i}$. This idea is illustrated in Figure S1 for three output modes.

In some applications, it may likewise be desirable to scatter several ($n$) orthogonal modes $\{u_i(t)\}_{i=1}^n$ on the quantum system. To model this, we consider a sequence of cascaded virtual input cavities with coupling strengths $g_{u_i}(t)$ and internal fields $\hat{a}_{u_i}$. The final of these directly ejects the first mode $u_1(t)$ towards the scatterer, while previous ones eject modes which are serially reflected on every cavity until the scatterer is reached. This is illustrated in Figure S1 for the case of three input modes.

The multi-mode extension of our theory thus incorporates $n+m$ virtual cavities, and the SLH formalism [S1]

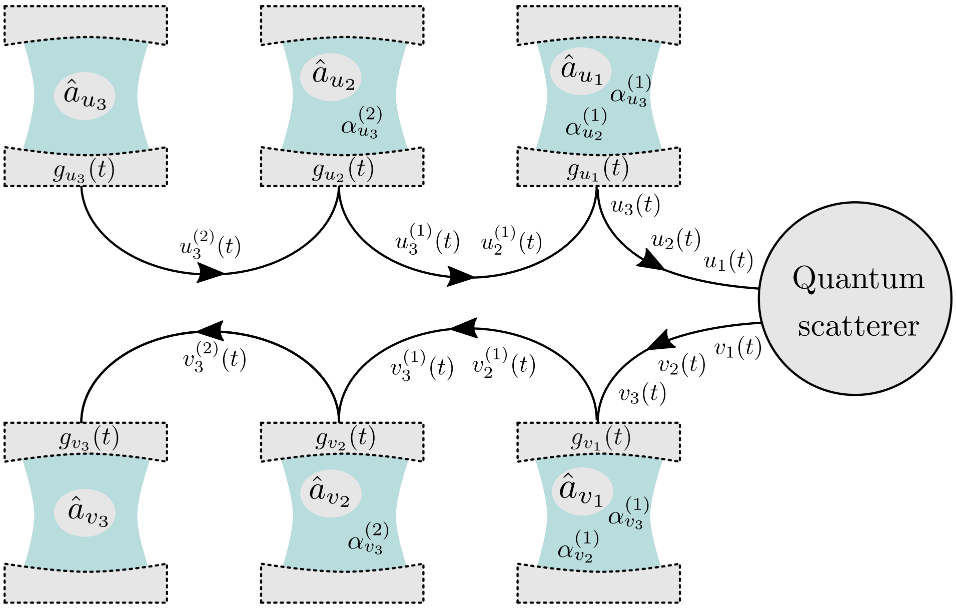


Figure S1. Illustration of the extension our formalism to include (for instance) $n = 3$ incoming modes, $u_1(t), u_2(t)$ and $u_3(t)$, and $m = 3$ outgoing modes $v_1(t)$, $v_2(t)$ and $v_3(t)$. The quantum state content of incoming (outgoing) mode $i$ is represented by a mode $\hat{a}_{u(v)_i}$ in a virtual cavity with coupling $g_{u(v)_i}(t)$. During the reflections, the modes are reshaped, and, e.g., input cavity three must emit the mode $u_3^{(2)}(t)$, which is transformed into $u_3^{(1)}(t)$ and subsequently into the desired $u_3(t)$ pulse incident on the scatterer (see main text of this supp. mat. for details).

* kiilerich@phys.au.dk
† moelmer@phys.au.dk

dictates that the full network evolves according to a Hamiltonian of the form

$$\hat{H}(t) = \hat{H}_{\mathrm{s}}(t) + \frac{i}{2}\left[\sum_{i=1}^{n} g_{u_i}^*(t)\hat{a}_{u_i}^\dagger \left(\sqrt{\gamma}\hat{c} + \sum_{j=1}^{i-1} g_{u_j}(t)\hat{a}_{u_j} + \sum_{i=1}^{m} g_{v_j}(t)\hat{a}_{v_j}\right) + \sum_{i=1}^{m}\left(\sqrt{\gamma^*}\hat{c}^\dagger + \sum_{j=1}^{i-1} g_{v_j}^*(t)\hat{a}_{v_j}^\dagger\right) g_{v_i}(t)\hat{a}_{v_i}\right]. \tag{S1}$$

and that a single Lindblad operator

$$\hat{L}_0 = \sqrt{\gamma}\hat{c} + \sum_{i=1}^{n} g_{u_i}(t)\hat{a}_{u_i} + \sum_{i=1}^{m} g_{v_i}(t)\hat{a}_{v_i} \tag{S2}$$

must be included along with separate damping and decoherence terms of the quantum scatterer in the master equation (4) of the main text.

To determine the the correct time dependent cavity coupling strengths $g_{v_i}(t)$ and $g_{u_i}(t)$ of the $n+m$ virtual cavities corresponding to the desired modes, we must take the distortion of each pulse shape by reflections on the subsequent sequence of cavities into account. Due to the linearity of the virtual cavity systems, this can be accomplished by the evolution of classical mode amplitudes. We emphasize that this task is performed prior to and independent of the solution of the ensuing quantum master equation. For completeness, we present below the derivation of the cavity couplings in detail.

### A. Coupling strengths for multiple outputs

In the scheme outlined above and illustrated in Figure S1, we must take into account that the output modes are reshaped by each reflection. That is, after the $j$th (virtual) cavity, the remaining modes are transformed as $v_i(t) \to v_i^{(j)}(t)$, where, since the reflection is a unitary process, the orthogonality between modes is preserved.

Let us considering the output mode $v_2(t)$. During the reflection of this mode on the first virtual cavity, the contribution $\alpha_{v_2}^{(1)}$ to the cavity field amplitude due to this particular pulse solves a differential equation

$$\dot{\alpha}_{v_2}^{(1)} = -g_{v_1}v_2 - \frac{|g_{v_1}|^2}{2}\alpha_{v_2}^{(1)} \tag{S3}$$

from an initial value $\alpha_{v_2}^{(1)}(0) = 0$. In Eq. (S3) and below, we omit the explicit time dependence of the rates and modes for simplicity of notation. The corresponding reflected mode amplitude is given by

$$v_2^{(1)} = v_2 + g_{v_1}^*\alpha_{v_2}^{(1)}. \tag{S4}$$

In order to associate the internal mode $\hat{a}_{v_2}$ of the second cavity with the mode $v_2(t)$, scattered from the quantum system, we should hence define the coupling rate of the second virtual cavity as [Eq. (3) of the main text]

$$g_{v_2}(t) = -\frac{\left[v_2^{(1)}(t)\right]^*}{\sqrt{\int_0^t dt'\,|v_2^{(1)}(t')|^2}}. \tag{S5}$$

Likewise, a third mode $v_3(t)$ contributes an amplitude in the first cavity given by

$$\dot{\alpha}_{v_3}^{(1)} = -g_{v_1}v_3 - \frac{|g_{v_1}|^2}{2}\alpha_{v_3}^{(1)}, \tag{S6}$$

and is rescattered to the second cavity as

$$v_3^{(1)} = v_3 + g_{v_1}^*\alpha_{v_3}^{(1)}. \tag{S7}$$

In the second cavity, a corresponding amplitude $\alpha_{v_3}^{(2)}(t)$ then builds up according to

$$\dot{\alpha}_{v_3}^{(2)} = -g_{v_2}v_3^{(1)} - \frac{|g_{v_2}|^2}{2}\alpha_{v_3}^{(2)} \tag{S8}$$

$$= -g_{v_2}\left(v_3 + g_{v_1}^*\alpha_{v_3}^{(1)}\right) - \frac{|g_{v_2}|^2}{2}\alpha_{v_3}^{(2)}, \tag{S9}$$

where we applied Eq. (S7) in the final equation. The reshaped mode, arriving at the third cavity, is $v_3^{(2)} = v_3^{(1)} + g_{v_2}^* \alpha_{v_3}^{(2)} = v_3 + g_{v_1}^* \alpha_{v_3}^{(1)} + g_{v_2}^* \alpha_{v_3}^{(2)}$, which defines the coupling strength $g_{v_3}(t) = -[v_3^{(2)}(t)]^* / \sqrt{\int_0^t dt' \, |v_3^{(2)}(t')|^2}$ to the associated cavity mode $\hat{a}_{v_3}$.

By now, the generalization to $m$ modes should be clear. For mode $1 < i \leq m$, we should solve $i-1$ coupled differential equations

$$\dot{\alpha}_{v_i}^{(j)} = -g_{v_j} \left( v_i + \sum_{k=1}^{j-1} g_{v_k}^* \alpha_{v_i}^{(k)} \right) - \frac{|g_{v_j}|^2}{2} \alpha_{v_i}^{(j)} \tag{S10}$$

for the associated amplitudes $\alpha_{v_i}^{(j)}(t)$ with $j = 1, 2, ..., i-1$ in each virtual cavity prior to the $i$th cavity.

Then, the mode in that cavity $\hat{a}_{v_i}$ captures precisely the quantum state of the original mode $v_i(t)$ if

$$g_{v_i}(t) = -\frac{\left[ v_i^{(i-1)}(t) \right]^*}{\sqrt{\int_0^t dt' \, |v_i^{(i-1)}(t')|^2}} \tag{S11}$$

with

$$v_i^{(i-1)} = v_i + \sum_{k=1}^{i-1} g_{v_k}^* \alpha_{v_i}^{(k)}. \tag{S12}$$

We note that with $m$ modes, one needs to solve $\sum_{i=1}^{m} (i-1) = m(m-1)/2$ differential equations for the needed amplitudes $\alpha_{v_i}^{(j)}(t)$. We imagine that the present formalism will not find relevance for $m$ larger than two or three.

### B. Coupling strengths for multiple inputs

As illustrated in Figure S1, the input modes similarly experience reflections which cause unitary transformations before they reach their final destination at the scatterer. By $u_i^{(j)}(t)$ we denote the shape of the mode $u_i(t)$ just *before* it is reflected on cavity $j$ (counting the cavities from the scatterer and out). In order to associate the field $\hat{a}_{u_i}$ in each cavity with a mode $u_i(t)$ *arriving* at the scatterer, the coupling strength $g_{u_i}(t)$ must thus be designed such that the mode $u_i^{(i-1)}(t)$, actually ejected from the $i$th towards the $(i-1)$th virtual cavity, correctly transforms into $u_i(t)$. That is [Eq. (2) of the main text]

$$g_{u_i}(t) = \frac{\left[ u_i^{(i-1)}(t) \right]^*}{\sqrt{1 - \int_0^t dt' \, |u_i^{(i-1)}(t')|^2}}. \tag{S13}$$

The $u_i^{(i-1)}(t)$ are determined by propagating backwards from the scatterer. For instance, a second mode $u_2(t)$ is ejected from the second virtual cavity as $u_2^{(1)}(t)$ and during reflection on the first cavity, the part of the mode entering has an amplitude $\alpha_{u_2}^{(1)}$, solving the equation

$$\dot{\alpha}_{u_2}^{(1)} = -g_{u_1} u_2^{(1)} - \frac{|g_{u_1}|^2}{2} \alpha_{u_2}^{(1)}. \tag{S14}$$

The reflected mode is required to produce the desired shape, i.e., $u_2 = u_2^{(1)} + g_{u_1}^* \alpha_{u_2}^{(1)}$. Under this condition, the equation may be rewritten

$$\dot{\alpha}_{u_2}^{(1)} = -g_{u_1} u_2 + \frac{|g_{u_1}|^2}{2} \alpha_{u_2}^{(1)}, \tag{S15}$$

and the mode $u_2^{(1)} = u_2 - g_{u_1}^* \alpha_{u_2}^{(1)}$, which should be used to define the rate (S13), identified.

For a third input mode $u_3(t)$, the corresponding mode $u_3^{(2)}(t)$, ejected from the third virtual cavity, is reflected on the second and first virtual cavitites before reaching the scatterer. During these reflections, amplitude contributions

$\alpha_{u_3}^{(2)}$ and $\alpha_{u_3}^{(1)}$ build up inside those cavities according to the equations

$$\begin{aligned}\dot{\alpha}_{u_3}^{(1)} &= -g_{u_1}u_3^{(1)} - \frac{|g_{u_1}|^2}{2}\alpha_{u_3}^{(1)} \\ \dot{\alpha}_{u_3}^{(2)} &= -g_{u_2}u_3^{(2)} - \frac{|g_{u_2}|^2}{2}\alpha_{u_3}^{(2)}.\end{aligned} \tag{S16}$$

The output from the first virtual cavity is given by $u_3^{(1)} + g_{u_1}^*\alpha_{u_3}^{(1)}$, and we require this to yield the desired mode, $u_3 = u_3^{(1)} + g_{u_1}^*\alpha_{u_3}^{(1)}$. At the same time, the input to the first cavity from the second cavity is given by $u_3^{(1)}(t) = u_3^{(2)} + g_{u_2}^*\alpha_{u_3}^{(2)}$. These two relations allow us to rewrite Eqs. (S16) in terms of the mode $u_3(t)$

$$\begin{aligned}\dot{\alpha}_{u_3}^{(1)} &= -g_{u_1}u_3 + \frac{|g_{u_1}|^2}{2}\alpha_{u_3}^{(1)} \\ \dot{\alpha}_{u_3}^{(2)} &= -g_{u_2}(u_3 - g_{u_1}^*\alpha_{u_3}^{(1)}) + \frac{|g_{u_2}|^2}{2}\alpha_{u_3}^{(2)}.\end{aligned} \tag{S17}$$

Upon solving the coupled differential equations (S17), the mode which defines the coupling $g_{u_3}(t)$ [Eq. (S13)] of the third cavity may be evaluated as $u_3^{(2)} = u_3 - g_{u_1}^*\alpha_{u_3}^{(1)} - g_{u_2}^*\alpha_{u_3}^{(2)}$.

Extending this line of thought reveals that $n$ input modes may be incorporated by solving $n(n-1)/2$ differential equations

$$\dot{\alpha}_{u_i}^{(j)} = -g_{u_j}\left(u_i - \sum_{k=1}^{j-1} g_{u_i}^*\alpha_{u_i^{(k)}}\right) - \frac{|g_{u_i}|^2}{2}\alpha_{u_i}^{(j)}, \tag{S18}$$

yielding the temporal mode shapes

$$u_i^{(i-1)} = u_i - \sum_{k=1}^{i-1} g_{u_k}^*\alpha_{u_i}^{(k)} \tag{S19}$$

which should be used to define the strengths Eq. (S13).

[S1] J. Combes, J. Kerckhoff, and M. Sarovar, "The SLH framework for modeling quantum input-output networks," Advances in Physics: X **2**, 784–888 (2017).
